# Supplementary material for: Search for $CP$ violation through an amplitude analysis of $D^0 \rightarrow K^+ K^- \pi^+ \pi^-$ decays
Source: arXiv:1811.08304 ancillary file (2019-03-06)
Supplement: Supplementary file 1 [file Lineshapes_Parametrisations.pdf]

# Ancillary material for LHCb-PAPER-2018-041

This document describes in detail the parametrisations of the amplitude analysis. In the isobar model [1, 2], which assumes that each amplitude can be built as a series of two-body decays, the two allowed patterns for  $D^0 \rightarrow abcd$ , both involving two intermediate resonances  $r_1$  and  $r_2$ , are the quasi two-body decay  $D^0 \rightarrow r_1 r_2$  followed by  $r_1 \rightarrow ab$  and  $r_2 \rightarrow cd$ , and the cascade decay  $D^0 \rightarrow r_1 a$  followed by  $r_1 \rightarrow r_2 b$  and  $r_2 \rightarrow cd$ . In both cases the amplitude is computed as

$$A(\mathbf{x}) = B'_{L_{D^0}}(q_{D^0}(\mathbf{x}), 0) \mathcal{T}_{r_1}(m_{r_1}(\mathbf{x}), L_{r_1}) \mathcal{T}_{r_2}(m_{r_2}(\mathbf{x}), L_{r_2}) W(\mathbf{x}), \quad (1)$$

where  $B'_{L_{D^0}}$  is the normalised Blatt–Weisskopf barrier factor [3] of the  $D^0$  candidate, given in Table 1. The function  $\mathcal{T}_r$  is the lineshape of resonance  $r$  and  $W$  is the spin factor, described with the covariant formalism [4]. The variable  $\mathbf{x}$  represents the five dimensions of the  $D^0 \rightarrow K^+ K^- \pi^+ \pi^-$  four-body phase space, and  $q_r$  is the magnitude of the momentum of one of the two daughter particles of resonance  $r$  in its rest frame. The variable  $m_r$  is the invariant mass of the daughter particles of resonance  $r$ , and  $L_r$  is the angular momentum between them.

## 1 Relativistic Breit–Wigner function

The default lineshape used for most resonances is the relativistic Breit–Wigner (RBW) function [5],

$$\mathcal{T}(m, L) = \frac{\sqrt{k} B'_L(q, 0)}{m_0^2 - m^2 - im_0 \Gamma(m, L)}, \quad (2)$$

where

$$\Gamma(m, L) = \Gamma_0 \left( \frac{q}{q_0} \right)^{2L+1} \left( \frac{m_0}{m} \right) B_L'^2(q, q_0), \quad (3)$$

is the running width of the resonance,  $m_0$  and  $\Gamma_0$  are the nominal values of the mass and width of the resonance, respectively, and  $q_0$  is the value of  $q$  when  $m = m_0$ . Indeed,  $q$  is a function of  $m$

$$q = \sqrt{\frac{m^2}{4} - \frac{m_1^2 + m_2^2}{2} + \frac{(m_1^2 - m_2^2)^2}{4m^2}}, \quad (4)$$

where  $m_1$  and  $m_2$  are the masses of the daughter particles. If one of the daughter particles is itself also a resonance, its mass ( $m_1$  or  $m_2$ ) is not fixed but depends on  $\mathbf{x}$ ; this adds an

Table 1: Normalised Blatt–Weisskopf barrier factors for the three first values of the angular momentum  $L$  between the decay products. The parameter  $R$  is the radius of the resonance.

| $L$ | $B'_L(q, q_0)$                                                             |
|-----|----------------------------------------------------------------------------|
| 0   | 1                                                                          |
| 1   | $\sqrt{\frac{1+q_0^2 R^2}{1+q^2 R^2}}$                                     |
| 2   | $\sqrt{\frac{(q_0^2 R^2 - 3)^2 + 9q_0^2 R^2}{(q^2 R^2 - 3)^2 + 9q^2 R^2}}$ |

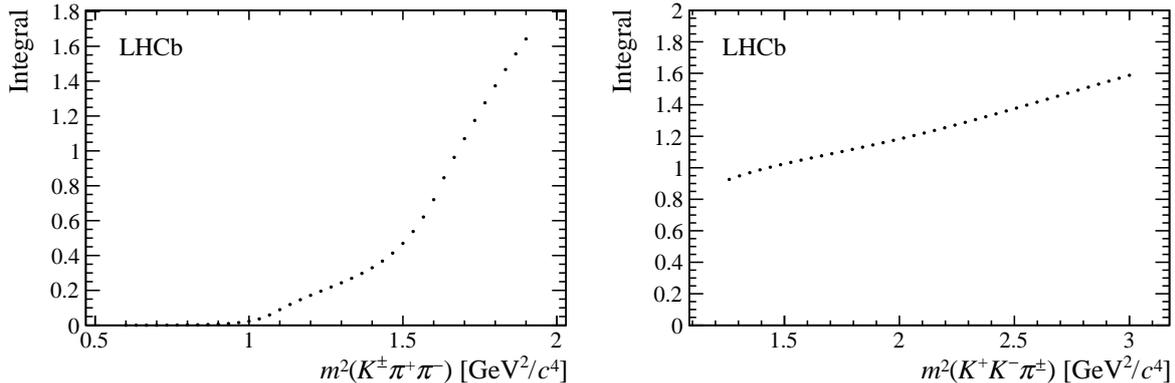

Figure 1: Cubic splines parametrising the integral of Eq. 6 for the  $K_1(1270)^\pm$  meson (left) and the  $a_1(1260)^\pm$  meson (right).

extra dependence on  $\boldsymbol{x}$  in the expression of the lineshape (not indicated in Eqs. 1 and 2). The factor  $k$  normalises the lineshape if the Blatt–Weisskopf form-factor and the energy dependence of the width are neglected, and reduces the correlations between the coupling to the channel and the mass and width of the resonance. It is given by

$$k = \frac{2\sqrt{2}m_0\gamma\Gamma_0}{\pi\sqrt{m_0^2 + \gamma}} \quad \text{with} \quad \gamma = m_0\sqrt{m_0^2 + \Gamma_0^2}. \quad (5)$$

The expression of the width given in Eq. 3 is not valid for the  $a_1(1260)^\pm$  and the  $K_1(1270)^\pm$  resonances, which both couple to various channels and resonances. Indeed, the finite widths of the intermediate resonances have an impact on the width of the mother. In this case a correction has to be implemented. Following the formalism presented in Ref. [6], the width is computed as an integral over the phase space of the three-body decay  $r \rightarrow abc$

$$\Gamma(m_r, L_r) \propto \frac{1}{m_r^2} \int |\mathcal{M}_{r \rightarrow abc}|^2 dm_{ab}^2 dm_{bc}^2, \quad (6)$$

where the integral is performed over the Dalitz plot, expressed in terms of the two-body invariant masses  $m_{ab}$  and  $m_{bc}$ , and the matrix element  $\mathcal{M}_{r \rightarrow abc}$  contains all contributing subdecays. For the  $K_1(1270)^\pm$  resonance, the integral is performed using the analysed dataset. However, since the  $a_1(1260)^\pm$  resonance is mainly decaying to three pions, the  $KK\pi$  channel is very small and not suitable to compute correctly this correction to the width. Its integral is therefore taken from a  $D^0 \rightarrow K^\mp \pi^\pm \pi^\pm \pi^\mp$  analysis [7], where the same formalism is used. The integrals are parametrised by interpolating cubic splines, which can then be exported and reused. The resulting splines describing the integrals over the analysed dataset are shown in Fig. 1.

Furthermore, the Blatt–Weisskopf form factors do not suppress the  $a_1(1260)^\pm$  and  $K_1(1270)^\pm$  width sufficiently as the mass of the decaying resonance grows, with the width eventually diverging. An exponential form factor derived from Ref. [6],

$$F(q) = e^{-R^2 q^2/2}, \quad (7)$$

is therefore used instead of  $B'_L(q, q_0)$  in Eq. 2.

## 2 Flatté distribution

The Flatté distribution [8] is used for the  $a_0(980)^0$  resonance near the  $KK$  threshold. In order to handle correctly the behaviour of the lineshape, it uses an analytical extension below the threshold. The  $a_0(980)^0$  meson couples to  $KK$  and  $\pi\eta$ , its width is thus affected by these two channels. This distribution is defined as

$$\mathcal{T}(m, L) = \frac{\sqrt{k}B'_L(q, 0)}{m_0^2 - m^2 - im_0(\Gamma_{KK}(m) + \Gamma_{\pi\eta}(m))} \quad (8)$$

with

$$\Gamma_{KK}(m) = g_{KK}^2 \sqrt{1 - \left(\frac{2m_K}{m}\right)^2}, \quad (9)$$

$$\Gamma_{\pi\eta}(m) = g_{\pi\eta}^2 \sqrt{\left[1 - \left(\frac{m_\pi + m_\eta}{m}\right)^2\right] \left[1 - \left(\frac{m_\pi - m_\eta}{m}\right)^2\right]}, \quad (10)$$

where the couplings  $g_{KK}^2 = 0.210 \pm 0.032 \text{ GeV}/c^2$  and  $g_{\pi\eta}^2 = 0.175 \pm 0.015 \text{ GeV}/c^2$  are taken from Ref. [9] and where  $m_\pi$  and  $m_\eta$  are taken from Ref. [10]. An analytical extension returns an imaginary width when the argument of the square root is negative. The normalisation factor  $k$  is the same as described in Eq. 5.

## 3 Gounaris–Sakurai distribution

The Gounaris–Sakurai parametrisation [11] is used for the  $\rho_0(770)^0$  meson decaying to two pions. This resonance is quite broad and is therefore not perfectly described by the RBW parametrisation. The lineshape is defined as

$$\mathcal{T}(m, L) = \frac{\sqrt{k}B'_L(q, 0)(1 + D\Gamma_0/m_0)}{m_0^2 - m^2 + f(m) - im_0\Gamma(m, L)}, \quad (11)$$

where the width  $\Gamma(m, L)$  is the same as in Eq. 3, the normalisation factor  $k$  is the same as in Eq. 5 and the constant  $D$  is given by

$$D = \frac{3m_\pi^2}{\pi q_0^2} \ln\left(\frac{m_0 + 2q_0}{2m_\pi}\right) + \frac{m_0}{2\pi q_0} - \frac{m_\pi^2 m_0}{\pi q_0^3}. \quad (12)$$

The function  $f(m)$  is given by

$$f(m) = \Gamma_0 \frac{m_0^2}{q_0^3} \left( q^2 (h(m) - h(m_0)) + q_0^2 \frac{m^2 - m_0^2}{2m} \frac{dh}{dm} \Big|_{m_0} \right), \quad (13)$$

$$h(m) = \frac{2}{\pi} \frac{q}{m} \ln\left(\frac{m + 2q}{2m_\pi}\right), \quad (14)$$

and where  $\frac{dh}{dm}$  is the total derivative of  $h$  with respect to  $m$ , taking into account that  $q = \sqrt{\frac{m^2}{4} - m_\pi^2}$ .

## 4 $\rho - \omega$ interference

The  $\rho(770)^0$  and the  $\omega(782)$  mesons are close in mass and interfere therefore heavily. The two separate resonances can be considered as a single state described by the superposition of the two individual states. During the model building, whenever a  $\rho(770)^0$  meson is added to the model, an  $\omega(782)$  meson is added as well. The  $\rho - \omega$  state is described as

$$|\rho - \omega\rangle = |\rho\rangle + \tilde{c}|\omega\rangle, \quad (15)$$

where  $\tilde{c}$  is a complex coefficient that is left floating in the fit.

## 5 K-matrix formalism

The RBW lineshape describes accurately well separated narrow resonances. In the case of broad overlapping resonances the K-matrix formalism [12] is used instead. Advantages of this formalism are a correct description of the interferences and compliance with unitarity. The K-matrix formalism describes the resonances by taking into consideration all the channels to which they couple. This is an important feature, since all the channels contribute to the width of the resonance. This formalism was traditionally used for scattering processes and is slightly modified in this analysis to be used for production processes. The lineshapes are defined as

$$\hat{\mathcal{T}} = \left( I - i\hat{K}\rho \right)^{-1} \hat{P}, \quad (16)$$

where  $I$  is the identity matrix and  $\rho$  is a diagonal phase-space matrix, which describes the behaviour of the various channels. For the two-body channels, the diagonal elements of  $\rho$  have the form [12]

$$\rho(m) = \sqrt{\left( \frac{m^2 - (m_1 + m_2)^2}{m^2} \right) \left( \frac{m^2 - (m_1 - m_2)^2}{m^2} \right)}, \quad (17)$$

where  $m_1$  and  $m_2$  are the daughter masses taken from Ref. [10]. The matrix  $\hat{K}$  is a  $n \times n$  matrix, with  $n$  being the number of channels to which the resonance couples. It describes both the resonant structure and the non-resonant scattering part of the amplitude. Finally,  $\hat{P}$  is the production vector. It has the same pole structure as the K-matrix, such that the amplitude does not vanish at the K-matrix poles. This formalism is used for the two components described in the next subsections.

### 5.1 $\pi\pi/KK$ S-waves

The  $\pi\pi$  and the  $KK$  S-waves are both described by the same K-matrix that couples to five different channels and five different poles. The parametrisation is taken from Ref. [13], where the K-matrix is defined as

$$\hat{K}_{ij}(m) = f(m) \left( \sum_{\alpha} \frac{g_{\alpha i} g_{\alpha j}}{m_{\alpha}^2 - m^2} + f_{ij}^{\text{scatt}} \frac{1 \text{ GeV}^2/c^4 - s_0^{\text{scatt}}}{m^2 - s_0^{\text{scatt}}} \right), \quad (18)$$

where  $i, j = 1, 2, 3, 4, 5$  indicate the channel and  $\alpha = 1, 2, 3, 4, 5$  indicates the pole. The channels are  $\pi\pi$ ,  $KK$ ,  $\pi\pi\pi\pi$ ,  $\eta\eta$  and  $\eta\eta'$ , while the poles are the  $f_0(980)$ ,  $f_0(1300)$ ,  $f_0(1500)$ ,  $f_0(1200 - 1600)$  and  $f_0(1750)$  resonances. The masses of the poles  $m_\alpha$  are [14]

$$m_\alpha = \begin{pmatrix} 0.651 \\ 1.2036 \\ 1.55817 \\ 1.21 \\ 1.82206 \end{pmatrix} \text{ GeV}/c^2. \quad (19)$$

The factors  $g_{\alpha i}$  are the coupling constants between the channel  $i$  and the pole  $\alpha$ . They have been measured from scattering data and their values are [14]

$$g_{\alpha i} = \begin{pmatrix} 0.22889 & -0.55377 & 0.00000 & -0.39899 & -0.34639 \\ 0.94128 & 0.55095 & 0.00000 & 0.39065 & 0.31503 \\ 0.36856 & 0.23888 & 0.55639 & 0.18340 & 0.18681 \\ 0.33650 & 0.40907 & 0.85679 & 0.19906 & -0.00984 \\ 0.18171 & -0.17558 & -0.79658 & -0.00355 & 0.22358 \end{pmatrix} \text{ GeV}/c^2. \quad (20)$$

The second term of Eq. 18 describes the non-resonant scattering contribution of the amplitude. The parameters needed are also taken from Ref. [14], where  $s_0^{\text{scatt}} = -3.93 \text{ GeV}^2/c^4$  and

$$f_{ij}^{\text{scatt}} = \begin{pmatrix} 0.23399 & 0.15044 & -0.20545 & 0.32825 & 0.35412 \\ 0.15044 & 0.00000 & 0.00000 & 0.00000 & 0.00000 \\ -0.20545 & 0.00000 & 0.00000 & 0.00000 & 0.00000 \\ 0.32825 & 0.00000 & 0.00000 & 0.00000 & 0.00000 \\ 0.35412 & 0.00000 & 0.00000 & 0.00000 & 0.00000 \end{pmatrix}. \quad (21)$$

The elements  $f_{ij}^{\text{scatt}}$  terms have only been measured for the scattering between the  $\pi\pi$  channel and the others, not among the other channels. There is a non-physical singularity below the  $\pi\pi$  threshold, sometimes called the ‘‘Adler zero’’, that is suppressed by the term  $f(m)$ . It is defined in Ref. [15] as

$$f(m) = \frac{1 \text{ GeV}^2/c^4 - s_{A0}}{m^2 - s_{A0}} \left( m^2 - s_A \frac{m_\pi^2}{2} \right), \quad (22)$$

where  $s_{A0} = -0.15 \text{ GeV}^2/c^4$  and  $s_A = 1$ . The phase-space term of the two-body channels ( $i = 1, 2, 4, 5$ ) is described in Eq. 17. The phase-space term for the four-pion channel ( $i = 3$ ) is

$$\rho_3(m) = \begin{cases} \sqrt{1 - \frac{(4m_\pi)^2}{m^2}} & \text{if } m \geq 1 \text{ GeV}/c^2, \\ \rho'_3(m) & \text{if } m < 1 \text{ GeV}/c^2, \end{cases} \quad (23)$$

where

$$\rho'_3(m) = \rho_0 \int \frac{dm_1^2}{\pi} \int \frac{dm_2^2}{\pi} \frac{M_0^2 \Gamma(m_1) \Gamma(m_2) \sqrt{(m^2 + m_1^2 - m_2^2)^2 - 4m^2 m_1^2}}{m^2 [(M_0^2 - m_1^2)^2 + M_0^2 \Gamma^2(m_1)] [(M_0^2 - m_2^2)^2 + M_0^2 \Gamma^2(m_2)]} \quad (24)$$

and  $\rho_0$  ensures that  $\rho_3(m)$  is continuous at  $m = 1 \text{ GeV}/c^2$ . The integration variables  $m_1^2$  and  $m_2^2$  are the squares of the invariant masses of the two di-pion states,  $M_0$  is the

Table 2: Parameters of the  $\pi\pi$  and  $KK$  K-matrices for all the relevant amplitudes. The moduli of the parameters  $\beta_\alpha$  are expressed in  $\text{GeV}/c^2$ .

| Amplitude                                          | Parameter                  | Modulus         | Phase [rad]      |
|----------------------------------------------------|----------------------------|-----------------|------------------|
| $D^0 \rightarrow [K^+K^-]_{L=0}[\pi^+\pi^-]_{L=0}$ | $f_{KK}^{\text{prod}}$     | 1 (fixed)       | 0 (fixed)        |
|                                                    | $K^+K^- \beta_1$           | $0.30 \pm 0.03$ | $0.43 \pm 0.09$  |
|                                                    | $K^+K^- \beta_2$           | $1.08 \pm 0.04$ | $1.38 \pm 0.03$  |
|                                                    | $f_{\pi\pi}^{\text{prod}}$ | 1 (fixed)       | 0 (fixed)        |
|                                                    | $\pi^+\pi^- \beta_1$       | $0.60 \pm 0.08$ | $-2.53 \pm 0.12$ |
| $D^0 \rightarrow (\rho - \omega)^0[K^+K^-]_{L=0}$  | $f_{KK}^{\text{prod}}$     | 1 (fixed)       | 0 (fixed)        |
|                                                    | $\beta_1$                  | $0.12 \pm 0.08$ | $2.59 \pm 0.82$  |
| $D^0 \rightarrow \phi(1020)[\pi^+\pi^-]_{L=0}$     | $f_{\pi\pi}^{\text{prod}}$ | 1 (fixed)       | 0 (fixed)        |
|                                                    | $\beta_1$                  | $2.54 \pm 0.51$ | $1.12 \pm 0.18$  |

pole mass of the  $\rho(770)^0$  resonance [10] and  $\Gamma(m) = \Gamma_0(1 - (4m_\pi^2/m^2))^{3/2}$  is the energy-dependent width, where  $\Gamma_0$  is set to  $0.3 \text{ GeV}/c^2$ . As shown in Ref. [16], the function  $\rho'_3(m)$  can be approximated by a 6th order polynomial in  $m^2$  (with  $m$  expressed in  $\text{GeV}/c^2$ )

$$\rho'_3(m) = 0.0005 - 0.0193m^2 + 0.1385m^4 - 0.2084m^6 - 0.2974m^8 + 0.1366m^{10} + 1.0789m^{12}. \quad (25)$$

The production vector is given by

$$\hat{P}_i(m) = \sum_\alpha \frac{\beta_\alpha g_{\alpha i}}{m_\alpha^2 - m^2} + f_i^{\text{prod}} \frac{1 \text{ GeV}^2/c^4 - s_0^{\text{prod}}}{m^2 - s_0^{\text{prod}}}, \quad (26)$$

where the complex parameter  $\beta_\alpha$  describes the production strength of pole  $\alpha$ , the complex parameter  $f_i^{\text{prod}}$  describes the direct coupling to channel  $i$  and  $s_0^{\text{prod}}$  is a single real parameter. The production vector therefore contains 21 free parameters that should be left floating in the fit. Despite the large data sample in the analysis, some of these parameters are not well constrained. In order to improve the fit stability during the model building, only the main component is kept, *i.e.* the direct coupling to the relevant channel ( $f_1^{\text{prod}}$  for the  $\pi\pi$  channel and  $f_2^{\text{prod}}$  for the  $KK$  channel). The direct couplings to the other channels ( $f_{3,4,5}^{\text{prod}}$ ) and to the poles ( $\beta_{1,2,3,4,5}$ ) are set to 0. All the poles and channels still contribute in the K-matrix computation of Eq. 18; their direct couplings are only removed from the production vector.

Once the model is built, all the pole couplings  $\beta_\alpha$  are tested. The fit does not converge if all the fit parameters are left floating in addition to these couplings. Therefore all the fit parameters are fixed to their nominal values and only the parameters of the K-matrix are fitted. The fit is not sensitive to all of them because the available phase space is relatively small. The direct coupling to  $f_0(980)$  is added to all the amplitudes containing a  $KK$  or  $\pi\pi$  S-wave and the coupling to  $f_0(1300)$  is only added to the  $KK$  K-matrix in the  $D^0 \rightarrow [K^+K^-]_{L=0}[\pi^+\pi^-]_{L=0}$  amplitude, because it is the only one where there is enough phase space. The contribution of the poles with higher masses ( $f_0(1500)$ ,  $f_0(1750)$  and  $f_0(1200 - 1600)$ ) is negligible. The decision of keeping the direct coupling to a pole or not is only based on the convergence or non-convergence of the fit. The values obtained, shown in Table 2, are then fixed in the main fit. The fit is only mildly sensitive to  $s_0^{\text{prod}}$ , with a preferred value in the range  $[-0.20, -0.07] \text{ GeV}^2/c^4$ . It is decided to fix  $s_0^{\text{prod}}$  to  $-0.17 \text{ GeV}^2/c^4$  for all the components.

## 5.2 $K\pi$ $S$ -wave

The  $K\pi$   $S$ -wave couples to two channels,  $K\pi$  and  $K\eta'$ , and contains only one pole, the  $K_0^*(1430)$  resonance. Two isospin states contribute to the  $K\pi$   $S$ -wave,  $I = \frac{1}{2}$ , which couples to both channels, and  $I = \frac{3}{2}$ , which couples to  $K\pi$  only. The parametrisation is taken from Ref. [17] and the K-matrix for  $I = \frac{1}{2}$  is given by

$$\hat{K}_{ij}^{\frac{1}{2}}(m) = \frac{m^2 - s_{0\frac{1}{2}}}{m_K^2 + m_\pi^2} \left( \frac{g_{1i}g_{1j}}{m_1^2 - m^2} + C_{ij0} + C_{ij1}\tilde{s} + C_{ij2}\tilde{s}^2 \right), \quad (27)$$

where the mass of the  $K_0^*(1430)$  pole is  $m_1 = 1.3386 \text{ GeV}/c^2$ , the Adler zero is located at  $s_{0\frac{1}{2}} = 0.23 \text{ GeV}^2/c^4$ , the couplings  $g_{1i}$  between the pole and the channels are

$$g_{1i} = \begin{pmatrix} 0.31072 \\ -0.02323 \end{pmatrix} \text{ GeV}/c^2, \quad (28)$$

and the coefficients of the second-order polynomial in  $\tilde{s} = \frac{m^2}{m_K^2 + m_\pi^2} - 1$  describing the non-resonant scattering contribution are

$$\begin{aligned} C_{ij0} &= \begin{pmatrix} 0.79299 & 0.15040 \\ 0.15040 & 0.17054 \end{pmatrix}, \\ C_{ij1} &= \begin{pmatrix} -0.15099 & -0.038266 \\ -0.038266 & -0.0219 \end{pmatrix}, \\ C_{ij2} &= \begin{pmatrix} 0.00811 & 0.0022596 \\ 0.0022596 & 0.00085655 \end{pmatrix}. \end{aligned} \quad (29)$$

The K-matrix for  $I = \frac{3}{2}$  does not couple to any resonance, it contains therefore only the non-resonant part

$$\hat{K}^{\frac{3}{2}}(m) = \frac{m^2 - s_{0\frac{3}{2}}}{m_K^2 + m_\pi^2} (D_{110} + D_{111}\tilde{s} + D_{112}\tilde{s}^2), \quad (30)$$

where the Adler zero is located at  $s_{0\frac{3}{2}} = 0.27 \text{ GeV}^2/c^4$  and

$$D_{110} = -0.22147, \quad D_{111} = 0.026637, \quad D_{112} = -0.00092057. \quad (31)$$

An approximation is made in order to describe the production vector of the  $K\pi$   $S$ -wave. It has been shown in Ref. [18] that, in a limited phase space, one can consider

$$\hat{K}^{-1}\hat{P} \approx \hat{\alpha}, \quad (32)$$

where  $\hat{\alpha}$  is a diagonal matrix containing a complex parameter for each channel, which is left floating in the fit. Therefore, the pole structure of the production vector cancels the pole structure of the K-matrix. This simplifies Eq. 16 to

$$\hat{\mathcal{T}} = \hat{T}\hat{K}^{-1}\hat{P} = \hat{T}\hat{\alpha}, \quad (33)$$

which describes the lineshape only in terms of the scattering process

$$\hat{T} = \left( I - i\hat{K}\rho \right)^{-1} \hat{K}. \quad (34)$$

Table 3: Parameters of the  $K\pi$  K-matrices for all the relevant amplitudes.

| Amplitude                                           | Parameter               | Modulus         | Phase [rad]      |
|-----------------------------------------------------|-------------------------|-----------------|------------------|
| $D^0 \rightarrow [K^+\pi^-]_{L=0}[K^-\pi^+]_{L=0}$  | $K^+\pi^- \alpha_{1/2}$ | 1 (fixed)       | 0 (fixed)        |
|                                                     | $K^+\pi^- \alpha_{3/2}$ | $0.31 \pm 0.02$ | $2.51 \pm 0.08$  |
|                                                     | $K^-\pi^+ \alpha_{1/2}$ | 1 (fixed)       | 0 (fixed)        |
|                                                     | $K^-\pi^+ \alpha_{3/2}$ | $0.36 \pm 0.02$ | $-2.95 \pm 0.05$ |
| $D^0 \rightarrow K^*(1680)^0[K^-\pi^+]_{L=0}$       | $\alpha_{1/2}$          | 1 (fixed)       | 0 (fixed)        |
|                                                     | $\alpha_{3/2}$          | $0.29 \pm 0.02$ | $-2.96 \pm 0.08$ |
| $D^0 \rightarrow \bar{K}^*(1680)^0[K^+\pi^-]_{L=0}$ | $\alpha_{1/2}$          | 1 (fixed)       | 0 (fixed)        |
|                                                     | $\alpha_{3/2}$          | $0.27 \pm 0.04$ | $-2.09 \pm 0.14$ |
| $K_1(1270)^+ \rightarrow [K^+\pi^-]_{L=0}, \pi^+$   | $\alpha_{1/2}$          | 1 (fixed)       | 0 (fixed)        |
|                                                     | $\alpha_{3/2}$          | $0.44 \pm 0.04$ | $-2.79 \pm 0.08$ |

The phase-space term of the  $K\pi$  K-matrix is described by Eq. 17.

Again, some assumptions are made while the model is being built. Only the dominant term is kept, which is the direct coupling to the  $K\pi$  channel in the isospin state  $I = \frac{1}{2}$ . Once the model is built, the direct coupling to the  $K\pi$  channel in the isospin state  $I = \frac{3}{2}$  as well as to the  $K\eta'$  channel are tested in all the amplitudes containing a  $K\pi$  S-wave. It turns out that the fit is not sensitive to the contribution of the  $K\eta'$  channel, so only the two isospin states of the  $K\pi$  channel are considered. Again, the fit does not converge if all the fit parameters are left floating in addition to the K-matrix parameters. Therefore all the fit parameters are fixed to the nominal values of the final model and the values of the K-matrix parameters are fitted. These parameters, shown in Table 3, are then fixed in the main fit.

## References

- [1] D. Herndon, P. Söding and R. J. Cashmore, *Generalized isobar model formalism*, Phys. Rev. **D11** (1975) 3165.
- [2] R. M. Sternheimer and S. J. Lindenbaum, *Extension of the isobaric nucleon model for pion production in pion-nucleon, nucleon-nucleon, and antinucleon-nucleon interactions*, Phys. Rev. **123** (1961) 333.
- [3] J. M. Blatt and V. F. Weisskopf, *Theoretical nuclear physics*, Chapter VIII.5, Springer, New York, 1952.
- [4] B. S. Zou and D. V. Bugg, *Covariant tensor formalism for partial-wave analyses of  $\psi$  decay to mesons*, Eur. Phys. J. **A16** (2003) 537, [arXiv:hep-ph/0211457](#).
- [5] G. Breit and E. Wigner, *Capture of slow neutrons*, Phys. Rev. **49** (1936) 519.
- [6] CLEO collaboration, D. M. Asner *et al.*, *Hadronic structure in the decay  $\tau^- \rightarrow \nu_\tau \pi^- \pi^0 \pi^0$  and the sign of the tau neutrino helicity*, Phys. Rev. **D61** (1999) 012002, [arXiv:hep-ex/9902022](#).
- [7] LHCb collaboration, R. Aaij *et al.*, *Studies of the resonance structure in  $D^0 \rightarrow K^\mp \pi^\pm \pi^+ \pi^-$  decays*, Eur. Phys. J. **C78** (2018) 443, [arXiv:1712.08609](#).
- [8] S. M. Flatté, *Coupled-channel analysis of the  $\pi\eta$  and  $K\bar{K}$  systems near  $K\bar{K}$  threshold*, Phys. Lett. **B63** (1976) 224.
- [9] V. V. Anisovich and A. V. Sarantsev, *The analysis of reactions  $\pi N \rightarrow 2$  mesons+N within reggeon exchanges. 1. Fit and results*, [arXiv:0806.1601](#).
- [10] Particle Data Group, M. Tanabashi *et al.*, *Review of particle physics*, Phys. Rev. **D98** (2018) 030001.
- [11] G. J. Gounaris and J. J. Sakurai, *Finite-width corrections to the vector-meson-dominance prediction for  $\rho \rightarrow e^+ e^-$* , Phys. Rev. Lett. **21** (1968) 244.
- [12] S. U. Chung *et al.*, *Partial wave analysis in K-matrix formalism*, Annalen der Physik **507** (1995) 404.
- [13] V. V. Anisovich and A. V. Sarantsev, *K-matrix analysis of the  $(IJ^{PC} = 00^{++})$ -wave in the mass region below 1900 MeV*, Eur. Phys. J. **A16** (2003) 229, [arXiv:hep-ph/0204328](#).
- [14] BaBar collaboration, B. Aubert *et al.*, *Improved measurement of the CKM angle  $\gamma$  in  $B^\mp \rightarrow D^{(*)} K^{(\mp)}$  decays with a Dalitz plot analysis of  $D$  decays to  $K_S^0 \pi^+ \pi^-$  and  $K_S^0 K^+ K^-$* , Phys. Rev. **D78** (2008) 034023, [arXiv:0804.2089](#).
- [15] S. L. Adler, *Sum rules for the axial-vector coupling-constant renormalization in  $\beta$  decay*, Phys. Rev. **140** (1965) B736, errata *ibid.* **149** (1966) 1294 and *ibid.* **175** (1968) 2224.

- [16] J. Back *et al.*, *LAURA<sup>++</sup>: A dalitz plot fitter*, Comput. Phys. Commun. **231** (2018) 198, [arXiv:1711.09854](#).
- [17] FOCUS collaboration, J. M. Link *et al.*, *Dalitz plot analysis of the  $D^+ \rightarrow K^- \pi^+ \pi^+$  decay in the FOCUS experiment*, Phys. Lett. **B653** (2007) 1, [arXiv:0705.2248](#).
- [18] R. N. Cahn and P. V. Landshoff, *Mystery of the  $\delta(980)$* , Nucl. Phys. **B266** (1986) 451.
